# Supplementary material for: Hydra: An Agentic Reasoning Approach for Enhancing Adversarial Robustness and Mitigating Hallucinations in Vision-Language Models
Source: arXiv:2504.14395 source file (2025-04-19)
Supplement: Supplementary file 1 [file 06-appendix.tex]

\section{Appendix}
%%%%%%%%%%%%%%%%%%%%%%%%%%%%%%
\mytodo{}
%%%%%%%%%%%%%%%%%%%%%%%%%%%%%%

\subsection{Hydra Workflow Illustrations}

\subsubsection{Hydra Workflow Illustrations - VQA Task}

\subsubsection{Hydra Workflow Illustrations - Captioning Task}

%%%%%%%%%%%%%%%%%%%%%%%%%%%%%%%%%%%%%%%%%%%%%%%%%%%%%%%%%
%%%%%%%%%%%%%%%%%%%%%%%%%%%%%%%%%%%%%%%%%%%%%%%%%%%%%%%%%
% next subsection
%%%%%%%%%%%%%%%%%%%%%%%%%%%%%%%%%%%%%%%%%%%%%%%%%%%%%%%%%
%%%%%%%%%%%%%%%%%%%%%%%%%%%%%%%%%%%%%%%%%%%%%%%%%%%%%%%%%

\subsection{Ablation Study}
%%%%%%%%%%%%%%%%%%%%%%%%%%%%%%
\mytodo{prolly remove this}
%%%%%%%%%%%%%%%%%%%%%%%%%%%%%%

%%%%%%%%%%%%%%%%%%%%%%%%%%%%%%%%%%%%%%%%%%%%%%%%%%%%%%%%%
%%%%%%%%%%%%%%%%%%%%%%%%%%%%%%%%%%%%%%%%%%%%%%%%%%%%%%%%%
% next subsection
%%%%%%%%%%%%%%%%%%%%%%%%%%%%%%%%%%%%%%%%%%%%%%%%%%%%%%%%%
%%%%%%%%%%%%%%%%%%%%%%%%%%%%%%%%%%%%%%%%%%%%%%%%%%%%%%%%%

\subsection{Prompt Templates}
